# Supplementary material for: Just Go with the Flow: Self-Supervised Scene Flow Estimation
Source: arXiv:1912.00497 source file (2020-04-13)
Supplement: Supplementary file 2 [file appendix.tex]

\paragraph*{Setup} We fine tune on KITTI dataset in a self-supervised manner using our model. Although KITTI provides ground truth scene flow annotations for the point clouds, we perform this experiment to test the generalization ability of our model. KITTI is a small-scale dataset and therefore to finetune on KITTI effectively, we initialize the network with the parameters of the model pre-trained on large-scale nuScenes dataset in a self-supervised manner as described above. For this set of experiments, we again train the model for 10K epochs with a batch size of 8. Since KITTI has scenes with two point clouds each, we simply pick the two point clouds as input to the model in each iteration. We experiment with different learning rates and augmentation of the training set with flipped point cloud sequences which we discuss later in this section. Once the training is complete, we use the scene flow prediction from the forward leg of our model to compute the EPE3D, ACC3D Strict, and ACC3D Relax for each experiment.
